# Supplementary material for: When to Call Your Neighbor? Strategic Communication in Cooperative Stochastic Bandits
Source: arXiv:2110.04396 source file (2021-10-08)
Supplement: Supplementary file 1 [file lowerBound_complete_graph.tex]

\noindent \textbf{Lower bound for regret.}
It has been established in \cite{lai1985asymptotically} that any asymptotically efficient algorithm (i.e.,  $\expe\left[n_k(T)\right]=o(T^a), \forall a>0$) at least pulls every arm logarithmically with time, i.e., $\expe\left[R(T)\right]=\Omega \left(\log T\right).$ Group regret of $N$ agents faced with the decentralized bandit problem for $T$ time steps is larger than the regret suffered by a single agent faced with the bandit problem for $TN$ time steps. Recall that each agent starts by pulling an arm randomly. Thus a lower bound for expected group cumulative regret can be given as  $\expe\left[R(T)\right]=\Omega\left(\log (TN)+N\right).$ For more information we refer reader to \cite{martinez2019decentralized}. This is a tight lower bound when communication network graph is complete. Deriving a graph structure dependent tight lower bound for a general graph becomes quite complicated due to the complexity of joint probability space of the agents. 

% \begin{remark} {\normalfont{(Tightness of lower bound)}}
% Aforementioned results provide a tight lower bound when communication network graph is complete. Deriving a graph structure dependent tight lower bound for a general graph becomes quite complicated due to the complexity of joint probability space of the agents. 
% Henceforth in this work for general graphs we restrict our focus to providing theoretical guarantees on upper bound and demonstrating validity our results through experiments.
% \end{remark}

\noindent \textbf{Specializing to complete communication graph.}
Recall that clique number of a complete graph is 1 and degree of all the vertices is $N-1$. Choose $\xi=\Bar{\xi}\frac{\log tN}{\log t},$ where $\Bar{\xi}>1.$ Then a modified uncertainty term can be given as 
\begin{align}
  C_k^{(i)}(t):=\sigma\sqrt{\frac{2\log (t^{\Bar{\xi}+1}N)}{N_k^{(i)}(t)}}. \label{eq:modun} 
\end{align}
Note that regret result provided in Theorem \ref{thm:regretB} linearly depends on the number of agents. Aforementioned modification to the uncertainty term allows us to obtain an improved bound for complete communication graph.

\begin{theorem}\label{thm:regretBComp}{{\normalfont{(Group regret of modified ComEx-UCB)}}} Consider a group of $N$ agents following ComEx-UCB with modified uncertainty term give in (\ref{eq:modun}), while sharing instantaneous rewards over a complete communication graph $G.$ Then for any $\Bar{\xi}\geq 1.1$ expected cumulative group regret satisfies:
\begin{align*}
 \expe &\left[R(T)\right] \leq\sum_{k=2}^K\frac{8(\Bar{\xi}+1)\sigma}{\Delta_k}\log \left(TN\right) +(N+3)\sum_{k=2}^K\Delta_k
\\
&+\frac{1}{N}\sum_{i=1}^N\left(12\log (3(d^{(i)}+1)) +3\log { (d^{(i)}+1)}\right)\sum_{k=2}^K\Delta_k
\end{align*}
\end{theorem}
\begin{proofsketch} We prove Theorem \ref{thm:regretBComp} by following a similar approach to proof of Theorem \ref{thm:regretB}. Note that we have $\Bar{\chi}(G)=1.$ Further since we modified the uncertainty term to include a $\log N$ term, i.e. see (\ref{eq:modun}), instead of a $\log T$ term we obtain $\log (TN)$ in the regret bound. However, this leads to an additional factor of $1/N$ for tail probability bound, which cancels out the factor $N$ we normally get by taking the summation over agents. A detailed proof of Theorem \ref{thm:regretBComp} is given below.
\end{proofsketch}

\begin{remark}
When communication graph is complete, corresponding regret bound for full communication can be given as $ \expe \left[R(T)\right]= O\left(\log (TN)+N\right)$ (Appendix H
). Thus from Theorem \ref{thm:regretBComp} we see that ComEx obtains the same order of performance as full communication. Recall that the lower bound for decentralized bandits is $ \expe \left[R(T)\right]= \Omega\left(\log (TN)+N\right).$ Thus our result is order optimal, i.e., matches the corresponding lower bound.
\end{remark}

\subsection{Proof of Theorem \ref{thm:regretBComp}}\label{sec:compregB}
Recall that when $G$ is a complete graph we have $\Bar{\chi}(G)=1.$ For $C_k^{(i)}(t)=\sigma\sqrt{\frac{2\log (t^{\Bar{\xi}+1}N)}{N_k^{(i)}(t)}},$ where $\Bar{\xi}>1,$ from Lemmas \ref{lem:tailrestate} and \ref{lem:RegDecomp} we have
\begin{align}
 \sum_{i=1}^N\expe[n^{(i)}_k(T)]  \leq  \eta_k+N+\sum_{i=1}^N\sum_{t=1}^{T-1}\left[\P \left(\widehat{\mu}_{1}^{(i)}(t)\leq \mu_{1}-C_{1}^{(i)}(t)\right)+\P \left(\widehat{\mu}_{k}^{(i)}(t)\geq \mu_{k}+C_{k}^{(i)}(t)\right)\right].\label{eq:regcom}
\end{align}
where $\eta_k=\frac{8(\Bar{\xi}+1)\sigma}{\Delta_k}\log (TN).$ Now we provide a tail probability bound to the results provided in Lemma \ref{lem:tailApp}.

\begin{lemma}{\bf{(Tail probability bound)}}\label{lem:tailAppcomp}
For some $\sigma\geq\sigma_k$ and for any $\zeta>1$ 
\begin{align*}
    \P\left(\Big|\widehat{\mu}_k^{(i)}(t)-{\mu}_k\Big |\geq \sigma\sqrt{\frac{2\log \left(t^{\Bar{\xi}+1}N\right)}{N_k^{(i)}(t)}}\right) \leq \frac{1}{N\log \zeta}\frac{\log (tN)}{t^{(\Bar{\xi}+1)\left(1-\frac{(\zeta-1)^2}{16}\right)}}
\end{align*}
\end{lemma}

\begin{proof}
\normalfont

We follow an similar approach to Lemma \ref{lem:tailApp}. Let $X_k$ be the sub-Gaussian random variable that models rewards drawn from arm $k.$ Then $X_k$ has mean $\mu_k$ and  variance proxy $\sigma_k.$ Define a new random variable such that $\forall \tau>0.$
\begin{align*}
Y_k^{(i)}(\tau)&=\left(X_k-\mu_k\right )\sum_{j=1}^N\indicate {A^{(i)}_\tau = k}\indicate {(i,j) \in E_{\tau} }.
\end{align*}
Let $Z_k^{(i)}(t)=\sum_{\tau=1}^{t}Y_k^{(i)}(\tau).$ For any $\lambda>0.$ Similar to the result provided in Lemma \ref{lem:tailApp} we have,
\begin{align*}
\expe\left(\exp\left(\lambda Z_k^{(i)}(t)-\frac{\lambda^2 \sigma_k^2}{2}N_k^{(i)}(t)\right)\right) \leq 1.
\end{align*}

Note that we have
\begin{align*}
\P\left(\exp\left(\lambda Z_k^{(i)}(t)-\frac{\lambda^2 \sigma_{k}^2}{2}N_k^{(i)}(t)\right)\geq \exp\left(2\kappa \vartheta\right)\right)=\P\left(\lambda Z_k^{(i)}(t)-\frac{\lambda^2 \sigma_k^2}{2}N_k^{(i)}(t)\geq 2\kappa \vartheta\right)\\
=\P\left(\frac{Z_k^{(i)}(t)}{\sqrt{N_k^{(i)}(t)}}\geq  
\frac{2\kappa\vartheta}{\lambda}\sqrt{\frac{1}{N_k^{(i)}(t)}}+\frac{\sigma_k^{2}}{2}\lambda \sqrt{N_k^{(i)}(t)}
\right)
\end{align*}

Recall that when $G$ is complete $d^{(i)}=N-1,\forall i\in [N].$ Let $\zeta>1.$ Then  $
1\leq N_k^{(i)}(t)\leq \zeta^{D_{t}}$
where $D_{t}=\frac{\log (tN)}{\log \zeta}.$ For $\lambda_{l}=\frac{2}{\sigma_k}\sqrt{\frac{\kappa\vartheta}{\zeta^{l-1/2}}}$ and $\zeta^{l-1}\leq N_k^{(i)}(t)\leq \zeta^{l}$ we have
\begin{align*}
\frac{2\kappa\vartheta}{\lambda_l}\sqrt{\frac{1}{N_k^{(i)}(t)}}+\frac{\sigma_{k}^{2}}{2}\lambda_l \sqrt{N^k_{i}(t)}=\sigma_k\sqrt{\kappa\vartheta}\left(\sqrt{\frac{\zeta^{l-1/2}}{N_k^{(i)}(t)}}+\sqrt{\frac{N_k^{(i)}(t)}{\zeta^{l-1/2}}}\right)\leq \sqrt{\vartheta},
\end{align*}
where $\kappa=\frac{1}{\sigma_k^2\left(\zeta^{\frac{1}{4}}+\zeta^{-\frac{1}{4}}\right)^2}.$

Then we have,
\begin{align*}
\P\left(\frac{Z_k^{(i)}(t)}{N_k^{(i)}(t)}\geq\sqrt{ \frac{\vartheta}{N_k^{(i)}(t)}}\right)\leq \sum_{l=1}^{D_{T}}\exp(-2\kappa\vartheta)
\end{align*}
Substituting $\vartheta=2\sigma_k^{2}\log \left(t^{\Bar{\xi}+1}N\right)$ we get
\begin{align*}
    \P\left(\Big|\widehat{\mu}_k^{(i)}(t)-{\mu}_k\Big |\geq \sigma_k\sqrt{\frac{2\log \left(t^{\Bar{\xi}+1}N\right)}{N_k^{(i)}(t)}}\right) \leq \frac{1}{N\log \zeta}\frac{\log (tN)}{t^{(\Bar{\xi}+1)\left(1-\frac{(\zeta-1)^2}{16}\right)}}.
\end{align*}
Since $\sigma\geq\sigma_k$ we have
\begin{align*}
    \P\left(\Big|\widehat{\mu}_k^{(i)}(t)-{\mu}_k\Big |\geq \sigma\sqrt{\frac{2\log \left(t^{\Bar{\xi}+1}N\right)}{N_k^{(i)}(t)}}\right) \leq \frac{1}{N\log \zeta}\frac{\log (tN)}{t^{(\Bar{\xi}+1)\left(1-\frac{(\zeta-1)^2}{16}\right)}}.
\end{align*}

This concludes the proof of Lemma \ref{lem:tailAppcomp}.
\end{proof}

The proof of Theorem \ref{thm:regretBComp} follows from (\ref{eq:regcom}), Lemmas \ref{lem:tailsum} and \ref{lem:tailAppcomp}.
